# Supplementary material for: Transfer Learning via Unsupervised Task Discovery for Visual Question Answering
Source: arXiv:1810.02358 source file (2019-04-07)
Supplement: Supplementary file 1 [file supplement.tex]

\appendix
\clearpage

\iffalse
% ====================================================================
\begin{figure*}[!t]
	\centering
	\includegraphics[width=0.9\linewidth] {supple_figures/model_comparison_with_std_vqa_all.png}
	%\vspace{-0.2cm}
	\caption{
		\textbf{Combining knowledge from VQA and external visual data.}
		Evaluation results on a test set containing both out-of-vocabulary answers and trained answers.
		The proposed model showed relatively lower performance on trained answers but significantly better performance on out-of-vocabulary answers.
		In total, the proposed model showed the best performance.}
	\label{supple_fig:vqa_all}
	\vspace{-0.2cm}
\end{figure*}
% ====================================================================
\fi

% ====================================================================
% tab:action_compare
\begin{table*}[!hb]\footnotesize
\centering
\caption{
\textbf{Learned mapping between a question and a task specification.}
We retrieved questions for each answer sets based on the similarity score between task specification vectors.
Results show that appropriate task specifications are regressed from each questions. 
No explicit supervision is used for mapping between questions and task specifications.
}
\vspace{0.2cm}
\scalebox{1.1}{
    \begin{tabular}
    	{
    		 @{}L{3.0cm}@{}| @{}L{11.0cm}@{}    
    	}    
        \hline    
        Answer set $\vart_s$ & Questions \vspace{0.02cm} \\
        \hline
        animal.n.01 & what type of animals are near the road? / what species of animals are these?\\
        building\_material.n.01 & what kind of material is the flooring made from? / what is the type of flooring made of? \\
        meat.n.01 & what kind of meat is next to the broccoli? / what kind of meat is next to the veggies? \\
        %organic\_process.n.01 & what are the giraffes doing? / what are the animals doing?\\
        liquid.n.01 & what kind of soda are the people drinking? / what type of soda are they drinking ? \\
        %plane\_figure.n.01 & what shape is the tall structure to the right? / what shape is the cloud above building?\\
        %room.n.01 & what room in the house is this cat laying in? / what room of a house is this?\\
        %athletic\_game.n.01 & what type of sport ball is shown? / what type of sport are the men participating in? \\
        %conveyance.n.03 & what kind of motor vehicle are they riding? / what type of vehicle is shown in the sign? \\
        %implement.n.01 & what utensil is in the person 's hand? / what utensil is laying next to the bread? \\
        plant.n.02 & what kind of flower is in the tall vase? / what kind of plant leaves are on the plate? \\
        plant\_organ.n.01 & what type of fruit is the animal eating? / what kind of fruit is the kid eating? \\
        structure.n.01 & what type of structure are they in? / what kind of building structure is she in? \\
        furniture.n.01 & what piece of furniture are the cats sitting on? / what furniture is the cat sitting on?\\
        slope.n.01 & is the man going uphill or downhill? / is the bus parked uphill or downhill? \\
        color.n.01 & what color is the trash bag? / what color is the garbage bag? \\
        consumption.n.01 & what are the cows doing? / what are the animals doing? \\
        %natural & what type of cloud formation is present? / what type of cloud is in the sky?\\    
        %\_phenomenon.n.01 & \\
        artifact.n.01 & what object is the cat laying under? / what type of structure are they in? \\
        fruit.n.01 & what type of fruit is the animal eating? / what type of fruit juice is on the counter?\\
        %geographic & what type of building is this picture taken in? / what type of building are they in?\\
        %\_point.n.01 & \\
        building.n.01 & what kind of building structure is she in? / what type of building is he standing in?\\
        hair.n.01 & what hairstyle does the surfer have ? / what type of hairstyle does this man have ? \\
        communication.n.02 & what type of language is on the buildings? / what type of language is on the signs?\\ 
        body\_of\_water.n.01 & what type of body of water is the man on? / what type of body of water is in photo?\\
        tool.n.01 & what utensil is in the person 's hand? / what utensil is laying next to the bread? \\    
        time\_period.n.01 & what kind of season is it? / what type of season is it? \\
        appliance.n.02 & what kind of appliance is the cat standing in? / what appliance is she standing next to? \\
        public\_transport.n.01 & what type of transportation is passing by? / what type of vehicle is shown in the sign?\\
        fabric.n.01 & what type of fabric are the bears made of? / what type of fabric is the chair made of? \\ 
        tree.n.01 & what kind of trees are under all that snow? / what type of trees are the tall ones? \\
        beverage.n.01 & what kind of soda is on the desk? / what kind of soda is in the bottle? \\
        home\_appliance.n.01 & what kind of appliance is the cat standing in? / what appliance is she standing next to?\\
        consumer\_goods.n.01 & what clothing item is this person wearing? / what clothing item is the girl wearing?\\
        cutlery.n.02 & what type of utensil is on the tray? / what utensil is under the fork?\\
        edible\_fruit.n.01 & what type of fruit is the animal eating? / what kind of fruit is the purple fruit? \\
        shape.n.02 & what shape are most of the windows? / what shape is the tall structure to the right?\\
        meal.n.01 & what meal of the day are these designed for? / what meal are these typically eaten for?\\
        sport.n.01 & which sport are they doing? / what type of sport ball is shown?\\
        \hline
    \end{tabular}
}
\label{tab:task_regression_sup} 
\end{table*}
% ====================================================================

\section{Weakly Supervised Task Regression}

This section describes how task regression is performed by \eqref{eq:pretrain} in the main paper.

\iffalse
Visual question answering (VQA), is usually formulated as a subsequent problem of reference and answering~\cite{yang2016stacked, fukui2016multimodal}, where the reference step make attention on a region that is relevant to a question and the answering perform visual recognition specified by a question.
Hereby, the pretrained conditional visual classifier could be used for the answering step.
The conditional visual classifier is trained to perform diverse visual recognition by putting appropriate task vector $\tau$, so it could be utilized to VQA by inferring a task vector from a question.
We call this problem a task regression, where a task vector should be regressed from a natural language question.
\fi

Let $\varq$ be a question from a VQA dataset and $\tau^*_\varq$ be a true task specification defined by a question.
Our intuition is that a task is defined by a mapping from visual inputs to a set of answers, which is represented by a conditional distribution $\prob_{\tau_\varq^*}(\vara | \varv)$.
As the task is defined by a conditional distribution, the objective of a task regression becomes to find a task specification vector $\tau_{\eta_\vqa}(\varq)$ that approximates this conditional distribution using a pretrained task conditional visual classifier $\prob_\theta(\vara|\varv, \tau_{\eta_\vqa}(\varq))$.
We can formulate this objective as a maximum log-likelihood, which is formally written as follows.
\begin{equation}
\mathbb{E}_{\prob(\varv|\varq)}
	\mathbb{E}_{\tau^*_\varq(\vara|\varv)}
		[\log \, \prob_\theta(\vara|\varv, \tau_{\eta_\vqa}(\varq))],
\end{equation}
where $\prob(\varv|\varq)$ is conditional distribution of visual features $\varv$ given a question $\varq$.

As we are interested in learning $\eta_\vqa$, which is a parameter of a question encoder working over all question $\varq$, we need to optimized the objective expected over the distribution of $\varq$, which is formally written as follows.

{\color{red}
\begin{equation}
\begin{split}
\mathbb{E}&_{\prob(\varq)}
\mathbb{E}_{\prob(\varv|\varq)}
	\mathbb{E}_{\tau^*_\varq(\vara|\varv)}
	[\log \, \prob_\theta(\vara|\varv, \tau_{\eta_\vqa}(\varq))]\\
&=
\mathbb{E}_{\prob(\varq)}
\mathbb{E}_{\prob(\varv_{\phi_\vqa}(\varI, \varq)|\varq)}
\mathbb{E}_{\tau^*_\varq(\vara|\varv_{\phi_\vqa}(\varI, \varq))}
[\log\, \prob_\theta(\vara|\varv_{\phi_\vqa}(\varI, \varq), \tau_{\eta_\vqa}(\varq))]\\
&=
\mathbb{E}_{\prob(\varq)}
\mathbb{E}_{\prob(\varI|\varq)}
\mathbb{E}_{\tau^*_\varq(\vara|\varI, \varq)}
[\log\, \prob_\theta(\vara|\varv_{\phi_\vqa}(\varI, \varq), \tau_{\eta_\vqa}(\varq))]\\
&=
\mathbb{E}_{\prob_\vqa(\vara, \varI, \varq)}
	[\log\, \prob_\theta(\vara|\varv_{\phi_\vqa}(\varI, \varq), \tau_{\eta_\vqa}(\varq))],
\end{split}
\end{equation}
}
where, $\prob_\vqa(\vara, \varI, \varq) = \tau^*_\varq(\vara|\varI, \varq)\prob(\varI|\varq)\prob(\varq)$ and a visual feature $\varv$ is altered to $\varv_{\phi_\vqa}(\varI, \varq)$ because the visual feature is inferred by a visual encoder from an image $\varI$.
This derivation relates the task regression to standard VQA objective in \eqref{eq:transfer} in the main paper.

\section{Additional Task Regression Results}
Table~\ref{tab:task_regression_sup} shows examples of task regressed questions corresponding to each answers sets, which are represented as the synset of common hypernyms.
Similarity is computed by dot product between task specification vector of the answer set embedding $\tau_{\eta_\pre}(\vart_s)$ and the task specification vector regressed by a question $\tau_{\eta_\vqa}(\mathbf{q})$.
We manually select top ranked questions that fit within the table in terms of the number of characters.

% ====================================================================
\begin{figure*}[!t]
	\centering
	\includegraphics[width=0.9\linewidth] {supple_figures/qualitative_diverse_type.jpg}
	%\vspace{0.1cm}
	\caption{
		\textbf{Out-of-vocabulary answers with diverse types of concepts.}
		Green and red color denote correct and wrong answers respectively. Asterisk~(*) denotes answers appearing in the training set. Answers without asterisks are out-of-vocabulary answers.
		The proposed model correctly predicts out-of-vocabulary answers for diverse visual recognition tasks.
	}
	\label{supple_fig:qualitative1}
\end{figure*}
\section{Additional Qualitative Results}
To illustrate that the proposed model could answer diverse questions with out-of-vocabulary answers, we present additional qualitative results.
Figure~\ref{supple_fig:qualitative1} illustrates that the proposed model correctly predicts out-of-vocabulary answers to diverse visual recognition tasks.
Figure~\ref{supple_fig:qualitative23} illustrates that the proposed model performs question and image dependent answering and could predict out-of-vocabulary answers depending on both image and question.

% ====================================================================
%\setcounter{figure}{12}
\begin{figure*}[!t]
	\centering
	\subfigure[
		\textbf{Same task with different out-of-vocabulary answers.}
		Pair of questions are asking similar visual recognition task.
		The proposed model correctly predict out-of-vocabulary answers depending on different images.	
	]{
		\includegraphics[width=0.90\linewidth] {supple_figures/qualitative_same_task_different_answer.jpg}
			\label{supple_fig:qualitative2}
	}
	\subfigure[
		\textbf{Same image with diverse tasks}
		This qualitative example visualizes diverse question answering for a single image.
		The proposed model correctly predicts out-of-vocabulary answers depending on the question.
	]{
		\includegraphics[width=0.90\linewidth] {supple_figures/qualitative_same_image_different_task.jpg}
			\label{supple_fig:qualitative3}
	}
	%\vspace{0.1cm}
	\caption{
		\textbf{Image and question dependent answering.}
		Green and red color denote correct and wrong answers respectively. Asterisk(*) denotes answers appearing in the training set. Answers without asterisks are out-of-vocabulary answers.
	}
	\label{supple_fig:qualitative23}
\end{figure*}
% ====================================================================
